# Supplementary material for: Verifying Reachability in Networks with Mutable Datapaths
Source: arXiv:1607.00991 source file (2016-07-04)
Supplement: Supplementary file 1 [file appendix.tex]

\section{Network Slices}
\label{appendix:slices}
In this appendix we show, using the abstract semantics described in \secref{sec:scalability}, that $\overline{\Omega}$-invariants verified on a network slice also hold for the entire network. First, observe that the abstract semantics define a network as a transition system, where processing a packet moves a network from one state to another. At each state the network can either chose to process a packet already within the network (\ie a packet that is being forwarded through the network) or have a host send a new packet. Since slices are subnetworks, slices are also transition systems. Given this observation, we build on prior work~\cite{symmetryandsurgery} to prove that proving $\overline{\Omega}$-invariants on slices is sufficient. In particular, this requires that we prove: (a) there exists a bisimulation~\cite{groote1992structured} between a network and a slice, and (b) show that $\overline{\Omega}$-invariants are equivalent in the slice and network.

\noindent\textbf{Existence of a Bisimulation} In \secref{sec:scalability}, we defined the network transitions system using a transition relation $\rightarrow_{\Omega}$. To show a bisimulation between a network's transition system $\rightarrow_{\Omega}$ and a slice's transition system $\rightarrow_{\overline{\Omega}}$ we need to find a symmetric equivalence relation $\sim$ such that for any transition $(p, l, s)\rightarrow_{\Omega} (p',l',s')$ there exists an equivalent transition $(\overline{p}, \overline{l}, \overline{s})\rightarrow_{\overline{\Omega}} (\overline{p}',\overline{l}',\overline{s}')$ in $\rightarrow_{\overline{\Omega}}$ such that $(p, l, s)\sim(\overline{p}, \overline{l}, \overline{s})$ and $(p',l',s')\sim(\overline{p}',\overline{l}',\overline{s}')$, \ie each transition in the original network has an equivalent transition in the slice and vice-versa. In our model it is safe to decompose $\sim$ into an equivalence relation for packet $\sim_P$, links $\sim_L$ and states $\sim_S$, such that $(p, l, s)\sim(\overline{p}, \overline{l}, \overline{s})$ if and only if $p\sim_P \overline{p}$, $l\sim_L \overline{l}$ and $s\sim_S \overline{s}$. Therefore, we need to show that packet closure and state closure impose natural relations between slices and the entire network.

First, define $\sim_S$ such that $s\sim_S \overline{s} \iff s(r) =  \overline{s}(r) \forall r\in\overline{R}$, \ie a state in the entire network is similar to a state in the slice if all the registers that appear in the slice have the same value in both. Next from state equivalence, we know that for any reachable state $s\in S$, there exists an equivalent state $\overline{s}\in \overline{S}$ such that $s\sim_S \overline{s}$ (by definition). State equivalence also provides us with as sequence of packet, link pairs in each, such that if sequence $(p_0, l_0), (p_1, l_1), \ldots (p_k, l_k)$ leads to state $s$ in the overall network, then $(\overline{p_0}, \overline{l_0}), (\overline{p_1}, \overline{l_1}), \ldots (\overline{p_k}, \overline{l_k})$ leads to state $\overline{s}$ in $\overline{\Omega}$. Define $\sim_P$ and $\sim_L$ such that for all such pairs of sequence, $p_0\sim_P \overline{p_0}$ and $l_0\sim_P \overline{l_0}$, for all $p\in \overline{P}$, $p\sim_P p$ (\ie packets in the slice are equivalent to themselves in the overall network), for all $l\in \overline{L}$, $l\sim_L l$ (\ie links in the slice are equivalent to themselves in the overall network). Finally, for any packet $p$ in the original network without an equivalent in the slice, define $p\sim_P \bot$ (\ie the packet is equivalent to the null packet), and similarly for links. The equivalence relations $\sim_P$, $\sim_S$ and $\sim_L$ impose a bisimulation: it is simple to see that any transition in the slice maps to the same transition in the original network. Any transition in the original network that can (after some steps) affect a register in the slice is equivalent to a similar transition in the slice due to state closure, finally any transition in the original network that does not affect the slice is equivalent to a null transition. Therefore, $\sim_P$, $\sim_L$, $\sim_S$ as described here impose a bisimulation between a network and any of its slices.

\noindent\textbf{Equivalence for $\overline{\Omega}$-invariants} Finally, we would like to show that proving an $\overline{\Omega}$-invariant $I$ on a slice $\overline{\Omega}$ is equivalent to proving it on $\Omega$. Observe that an isolation (reachability) invariant states that some packet meeting some preconditions cannot be delivered to a particular node. Equivalently, this implies that an invariant holds if and only if no sequence of transitions from an initial state (where all registers are set to their default value) can reach a violating state. Therefore, we need to show that such a sequence of transitions exists in $\overline{\Omega}$ if and only if it exists in $\Omega$. This is a simple consequence of three facts: (a) as above we have established a bisimulation between $\Omega$ and $\overline{\Omega}$, such that a transition in one has an equivalent transition in the other, (b) due to packet closure, a sequence of transitions within the slice never escape the slice by construction, and (c) $\sim_P$, and $\sim_L$ are the identity relation for any packets or links in $\overline{\Omega}$ and the state equivalence relation $\sim_S$ is merely a restriction to those registers contained within the slice. The former two show a given sequence exists in the overall network if and only if an equivalent sequence exists in the slice (a SMT solver in the model can be thought of as a tool which finds such a sequence). The last fact allows us to transfer $\overline{\Omega}$-invariants from the whole network to a slice without modifying any of the constants, and thus proves the equivalence.

Therefore, given an appropriate slice $\overline{\Omega}$, any $\overline{\Omega}$ holds for the whole network $\Omega$ if and only if it also holds in the slice.
